# Supplementary material for: RACE: RoPE-Aligned Attention Compression Based on Query-Key Activation Energies
Source: arXiv:2610.28385 source file (2026-10-20)
Supplement: Supplementary file 1 [file additional_complementary.tex]

% Please add the following required packages to your document preamble:
% \usepackage[table,xcdraw]{xcolor}
% Beamer presentation requires \usepackage{colortbl} instead of \usepackage[table,xcdraw]{xcolor}
\begin{table}[]
\caption{
}
% \vspace{0.25cm}
\label{tab:add_complementary}
\centering
\resizebox{0.6\columnwidth}{!}{%
\begin{tabular}{ccccccccccccc}
\hline
\rowcolor[HTML]{EFEFEF} 
\textbf{Method}                                                      &  & \multicolumn{3}{c}{\cellcolor[HTML]{EFEFEF}\textbf{H2O: KV Size 256}} & \textbf{} & \multicolumn{3}{c}{\cellcolor[HTML]{EFEFEF}\textbf{SnapKV: KV Size 256}} & \textbf{} & \multicolumn{3}{c}{\cellcolor[HTML]{EFEFEF}\textbf{KIVI 2 bits}} \\
\textbf{\begin{tabular}[c]{@{}c@{}}Head Dim\\ Retained\end{tabular}} &  & 100\%                 & 75\%                  & 50\%                  &           & 100\%                  & 75\%                   & 50\%                   &           & 100\%                & 75\%                & 50\%                \\ \hline
\rowcolor[HTML]{EFEFEF} 
\textbf{wikitext (ppl)}    &  & 13.62                 & 15.12                 & 21.81                 &           & 12.76                  & 15.66                  & 18.44                  &           & 15.7                 & 16.58               & 17.14               \\
\textbf{hellaswag}                                                       &  & 0.66                  & 0.65                  & 0.62                  &           & 0.68                   & 0.65                   & 0.62                   &           & 0.69                 & 0.66                & 0.64                \\
\rowcolor[HTML]{EFEFEF} 
\textbf{piqa}                                                        &  & 0.85                  & 0.83                  & 0.79                  &           & 0.85                   & 0.83                   & 0.79                   &           & 0.86                 & 0.84                & 0.8                 \\
\textbf{arc\_challenge}                                                      &  & 0.48                  & 0.45                  & 0.42                  &           & 0.48                   & 0.45                   & 0.46                   &           & 0.48                 & 0.48                & 0.44                \\
\rowcolor[HTML]{EFEFEF} 
\textbf{boolq}                                                       &  & 0.79                  & 0.78                  & 0.71                  &           & 0.81                   & 0.79                   & 0.74                   &           & 0.78                 & 0.78                & 0.74                \\
\textbf{MMLU College CS}      &  & 0.66                  & 0.63                  & 0.4                   &           & 0.7                    & 0.63                   & 0.44                   &           & 0.7                  & 0.63                & 0.42                \\ \hline
\rowcolor[HTML]{EFEFEF} 
\textbf{Avg Acc}                                                     &  & 0.688                 & 0.668                 & 0.588                 &           & 0.704                  & 0.67                   & 0.61                   &           & 0.7                  & 0.63                & 0.42                \\ \hline
\end{tabular}
}
\end{table}
